# Supplementary material for: Bayesian Inverse Graphics for Few-Shot Concept Learning
Source: arXiv:2409.08351 source file (2024-09-12)
Supplement: Supplementary file 1 [file supplementary_differentiable_rendering.tex]

\begin{figure}[htpb]
    \begin{subfigure}[T]{0.50\linewidth}
        \includegraphics[width=\linewidth]{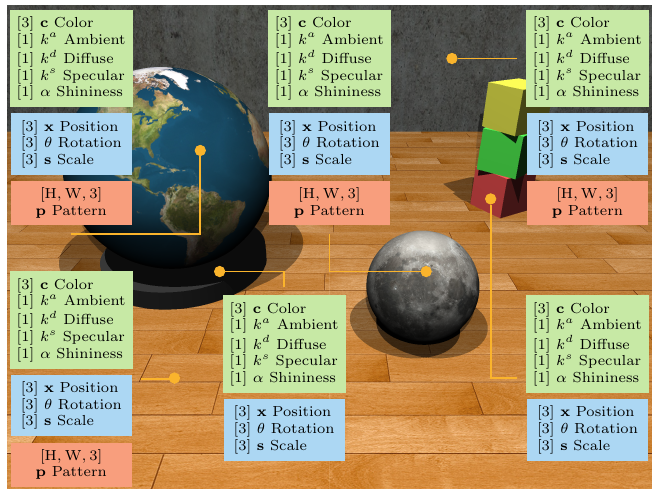}
        \caption{Example of differentiable scene parameters with their respective dimension sizes}~\label{fig:differentiable_rendering_parameters}
    \end{subfigure}
    \begin{subfigure}[T]{0.50\linewidth}
        \input{sections/images/differentiable_rendering_pipeline}
        \caption{Differentiable rendering pipeline}~\label{fig:differentiable_scene_optimization}
    \end{subfigure}
    \caption{Model based scene optimization}~\label{fig:model_based_optimization2}
\end{figure}
